# Supplementary material for: Theoretical analysis of glide-Z_2 magnetic topological photonic crystals
Source: arXiv:2109.01298 ancillary file (2021-09-03)
Supplement: Supplementary file 1 [file supplemental-document-210824.pdf]

# Theoretical analysis of glide- $Z_2$ magnetic topological photonic crystals: supplemental document

This supplemental document includes some details and tables used in the calculations in the main text.

## 1. Discussion on symmetry and topology of the topological photonic crystal

In this section, we discuss details of the similarities between the photonic crystals in this paper and the Kane-Mele model in electronic systems, discussed briefly in Sec. 2.2 in the main text. Compared with the case with  $\kappa = 0$  preserving TRS in Fig. S1(b), by breaking the TRS the band gap opens between the bands 2 and 3 at the  $P$  points, shown in (a) and (c) with  $\kappa_{(111)} = \pm 10i$ . The case with  $\kappa_{(111)} = +10i$  is found to be topological in Ref. [1], and because of the TRS, the other case with  $\kappa_{(111)} = -10i$  is also topological. The key to open the gap and to realize the topological phase is the splitting of the four-fold degenerate generalized Dirac point at the  $P$  point. Meanwhile, as we see later, the irreps at the  $P$  points do not affect the values of the topological invariant. It is consistent with the fact that the topological surface states appear both in  $\text{Im}(\kappa_{(111)}) > 0$  and in  $\text{Im}(\kappa_{(111)}) < 0$ , because the two sides  $\text{Im}(\kappa_{(111)}) > 0$  and  $\text{Im}(\kappa_{(111)}) < 0$  are related by time-reversal symmetry. This situation is similar to the Kane-Mele model (Figs. S1(d)-(f)), which is a tight-binding model on a honeycomb lattice in the  $xy$  plane with spin-orbit interaction [2, 3], showing the two-dimensional topological insulator (TI) phase with TRS:

$$H = t \sum_{\langle i,j \rangle} c_i^\dagger c_j + i\lambda_{so} \sum_{\langle\langle i,j \rangle\rangle} c_i^\dagger (\mathbf{s} \cdot \hat{\mathbf{e}}_{ij}) c_j, \quad (\text{S1})$$

where  $t$  and  $\lambda_{so}$  are real parameters,  $c_i^\dagger = (c_{i\uparrow}^\dagger, c_{i\downarrow}^\dagger)$  are creation operators for up-spin and down-spin electrons at the  $i$ -th site in the honeycomb lattice,  $\langle i, j \rangle$  denotes a pair of nearest neighbor sites, and  $\langle\langle i, j \rangle\rangle$  denotes a pair of next nearest neighbor sites.  $\mathbf{s} = (s_x, s_y, s_z)$  are the Pauli matrices. The first term is a nearest-neighbor hopping term, and the second term represents spin-orbit interaction for next-nearest neighbor hopping with  $\hat{\mathbf{e}}_{ij} = (\mathbf{d}_{ij}^1 \times \mathbf{d}_{ij}^2) / |\mathbf{d}_{ij}^1 \times \mathbf{d}_{ij}^2|$ , where  $\mathbf{d}_{ij}^1$  and  $\mathbf{d}_{ij}^2$  are vectors of the bonds in the honeycomb lattice constituting the next-nearest neighbor hopping from site  $j$  to site  $i$ . When  $\lambda_{so}$  is nonzero, Dirac points at the  $K$  and  $K'$  points in the BZ become gapped and the system becomes a 2D TI, regardless of the sign of  $\lambda_{so}$ . The  $Z_2$  topological invariant for the 2D TI is nontrivial, because the product of the parities at four TRIM ( $\Gamma$  and  $3M$  points in the BZ) in this model is  $-1$ , as addressed in Ref. [4]. Thus, the  $Z_2$  topological invariant does not depend on the irreps at the  $K$  point. Thus, topological properties in the BPI photonic crystal are similar to those in the Kane-Mele model. The BPI photonic crystal is topological, regardless of the sign of the magnetization represented by  $\kappa$ , which opens the gap at the  $P$  point. Likewise, the Kane-Mele model is topological, regardless of the sign of the spin-orbit coupling  $\lambda_{so}$ , which opens the gap at the  $K$  point. In both cases, the topological invariant is independent of the irreps at  $P$  or  $K$  points, because these points are not time-reversal invariant momenta (TRIM).

Here we note that their similarity is limited to the point discussed above, and they are quite different in other aspects. For example, their topological phases are different. The BPI photonic crystal is in the glide- $Z_2$  topological phase protected by the glide symmetry, while the Kane-Mele model is in the  $Z_2$  topological insulator phase protected by the time-reversal symmetry. Therefore, corresponding topological properties such as surface states are different.

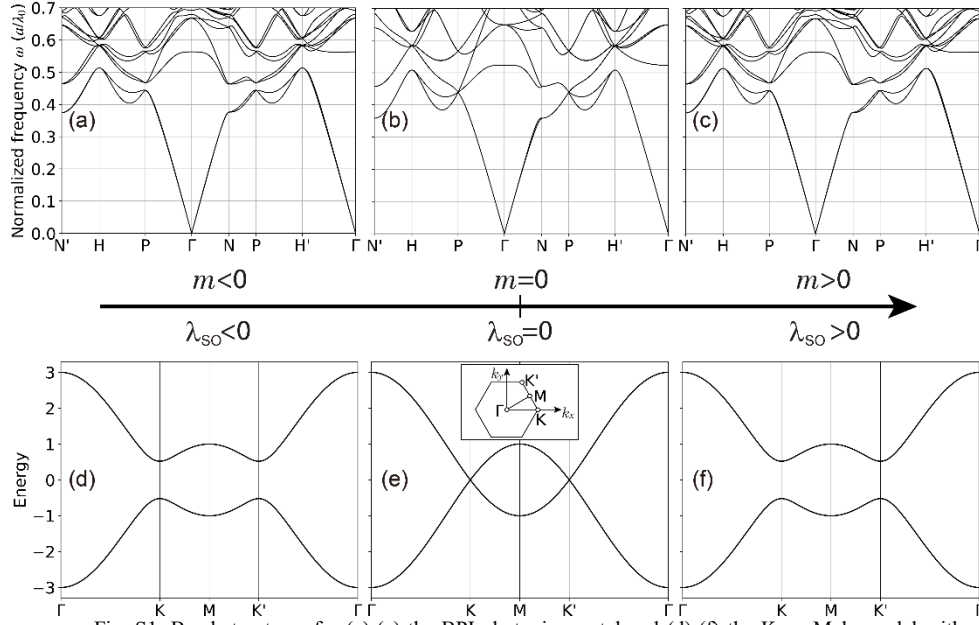

Fig. S1. Band structures for (a)-(c) the BPI photonic crystal and (d)-(f) the Kane-Mele model with inversion symmetry. The band structures with magnetization, where (a)  $\epsilon_{33} = 11$  and  $\kappa = 10i, 10i, -10i, -10i$  and (c) with  $\epsilon_{33} = 11$  and  $\kappa = -10i, -10i, 10i, 10i$  for the red, yellow, green and blue rods shown in (a), respectively, are exactly the same, because of the TRS, and both sides are topological. This situation is similar to the Kane-Mele model with changing the spin-orbit coupling across  $\lambda_{so}$  across zero, and the system is topological both for the positive  $\lambda_{so}$  and the negative  $\lambda_{so}$ . The parameter values are  $t = 0$  and (d)  $\lambda_{so} = -0.1$ , (e)  $\lambda_{so} = 0$ , and (f)  $\lambda_{so} = 0.1$ . The high-symmetry points for the BPI photonic crystal are shown in (c), whereas those for the Kane-Mele model are shown in the inset of (e), denoting the Brillouin zone of the honeycomb lattice.

## 2. GLIDE- $Z_2$ INVARIANT FOR THE PHOTONIC CRYSTAL

In this section, we discuss details of the derivation of the formula of the  $Z_2$  topological invariant for the cubic photonic crystals in Eq. (3) in Sec.3.3 of the main text. In magnetic glide-symmetric systems, the glide- $Z_2$  topological invariant can be defined, which characterizes a topological crystalline insulator phase [5-7]. Here we first review the definition of the glide- $Z_2$  topological invariant, and then we apply the formula to the photonic crystals. Let us begin with the SG 7 ( $Pc$ ) generated by the glide operation  $\hat{G}_y = \{M_y | (c/2)\hat{z}\}$  and translations  $\{E|a\hat{x}\}$ ,  $\{E|b\hat{y}\}$ , and  $\{E|c\hat{z}\}$  in a monoclinic primitive lattice, where we define  $a$ ,  $b$  and  $c$  to be the lattice constants along the  $x$ ,  $y$ , and  $z$  axes, respectively. In SG 7, we can define the glide- $Z_2$  invariant  $\nu$  as [5-7]

$$\nu = \frac{1}{2\pi} \left[ \int_A F_{xy} dk_x dk_y + \int_B F_{zx}^- dk_z dk_x - \int_C F_{zx}^+ dk_z dk_x \right] - \frac{1}{\pi} (\gamma_{A'BA}^+ + \gamma_{EDE'}^-) \pmod{2}, \quad (S2)$$

where  $A$ ,  $B$ , and  $C$  are the regions shown in Fig. S2(a). The superscript  $(\pm)$  indicates the glide sectors with eigenvalues of the glide operator  $g_{\pm} = \pm e^{-ik_z c/2}$  in spinless systems, such as photonic systems.  $F_{ij}^{\pm}(\mathbf{k})$  is the corresponding Berry curvatures for these subspaces  $F_{ij}^{\pm}(\mathbf{k}) = \partial_{k_i} A_j^{\pm}(\mathbf{k}) - \partial_{k_j} A_i^{\pm}(\mathbf{k})$ , and  $\gamma_{\lambda}^{\pm}$  is the corresponding Berry phase within the  $g_{\pm}$ -sector along the path  $\lambda$ ,  $\gamma_{\lambda}^{\pm} = \oint_{\lambda} \mathbf{A}^{\pm}(\mathbf{k}) \cdot d\mathbf{k}$ .  $\mathbf{A}^{\pm}(\mathbf{k})$  is the corresponding Berry connections given by the eigenstates  $|u_{nk}^{\pm}\rangle$ :  $\mathbf{A}^{\pm}(\mathbf{k}) \equiv i \sum_{n:occ} \langle u_{nk}^{\pm} | \nabla_{\mathbf{k}} | u_{nk}^{\pm} \rangle$ , where the band index  $n$  runs over the bands

below the gap considered. For fermions, this sum is over the occupied band indices. The Berry-phase terms  $\gamma_{A'B A}^+$ ,  $\gamma_{E D E'}^-$  in Eq. (S2) are along the paths  $A' \rightarrow B \rightarrow A$ , and  $E \rightarrow D \rightarrow E'$ . The value of  $\nu$  is either  $\nu = 0$  or  $\nu = 1$ , corresponding to the topologically trivial and nontrivial phases, respectively.

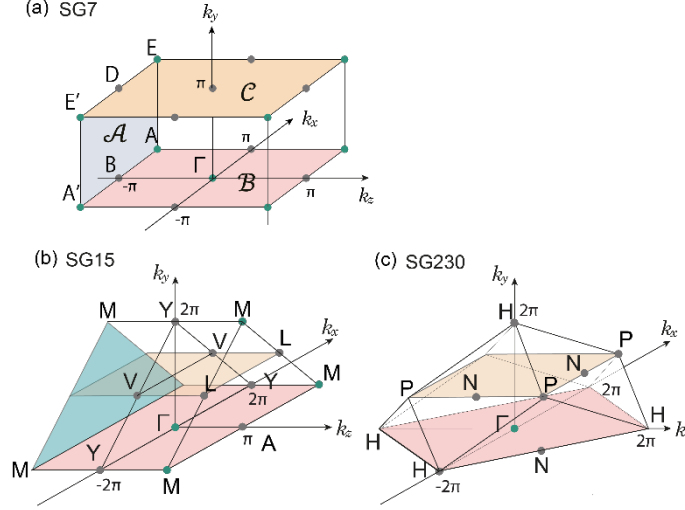

Fig. S2. (Color online) Brillouin zones for the SGs **7**, **15** and **230**. (a) Upper half of the Brillouin zone of the monoclinic simple lattice in **7** ( $Pc$ ). (b) Upper half of the Brillouin zone of the monoclinic base-centered lattice in **15** ( $C2/c$ ).  $\Gamma$ ,  $Y$ ,  $V$ ,  $A$ ,  $M$ , and  $L$  denote the high-symmetry points in SG **15**. (c) Upper half of the Brillouin zone of the body-centered cubic lattice in **230** ( $Ia3d$ ).  $\Gamma$ ,  $P$ ,  $H$ , and  $N$  denote the high-symmetry points in SG **230**. Here, for comparison, all the lattice constants are set to be unity.

Our target in the present paper is the photonic crystals in the BCC lattice, which is a nonprimitive lattice. As revealed in our previous paper [8], the nonprimitive nature of the lattice makes the formula of the  $Z_2$  topological invariant crucially different from that in the primitive lattice in **7**. Therefore, we here explain our results in the previous paper [8] for the nonprimitive lattice, for an application to the photonic crystals. By adding another translation  $\{E | \frac{1}{2}(a\hat{x} + b\hat{y})\}$ , the space group **7** becomes **9** ( $Cc$ ) in a monoclinic base-centered (nonprimitive) lattice. The formula for the glide- $Z_2$  topological invariant in the space group **9** is expressed in terms of integrals in the  $k$ -space found in Ref. [8], and it is still not easy to evaluate. Meanwhile, in the presence of inversion symmetry, like the photonic crystals of our interest, its formula is solely expressed in terms of the irreps at high-symmetry points, and is much easier to evaluate. In this case the space group becomes **15**, and the formula is obtained as [8]

$$(-1)^\nu = \prod_{i \in occ} \zeta_i^+(\Gamma) \xi_i^-(V) \frac{\xi_i^-(Y)}{\zeta_i^+(Y)}, \quad (S3)$$

where  $\zeta_i^+$  is a  $C_2$  eigenvalue in the  $g_+$  sector,  $\xi_i^-$  is an inversion parity for the  $i$ -th occupied state, and the product runs over the bands below the gap considered. We note that in the expressions of the glide- $Z_2$  topological invariant in Eq. (S3), the glide sectors with  $g_\pm = \pm e^{-ik_z c/2}$  can be switched. Namely, one can replace  $\zeta^+$  with  $\zeta^-$  in Eq. (S3).

Then, one can directly calculate the glide- $Z_2$  invariant in **230** by using Eq. (S3), because **15** is one of the  $t$ -subgroups of **230** [9], and their high-symmetry points are directly related with each other. The high-symmetry points  $\Gamma, Y$ , and  $V$  in **15** in Eq. (S3) are projections of  $\Gamma$ ,  $H$ , and  $N$  in **230**, respectively, as seen from the Brillouin zones for **15** in Fig. S2(b) and for **230** in Fig. S2(c). Here we assume that there exists a band gap between the second and third bands when

TRS is broken by applying a magnetic field, and from Eq. (S3), the glide- $Z_2$  topological invariant for this band gap is given by

$$(-1)^{\nu} = \prod_{i \in \text{occ}} \zeta_i^+(\Gamma) \xi_i(N) \frac{\xi_i(H)}{\zeta_i^+(H)},$$

where the product is taken over the bands below the gap considered. Remark (S4) **230**, the formula (S4) for the  $Z_2$  topological invariant is further simplified drastically, by evaluating Eq. (S4) term by term. First, the  $H$  point has three possible physically irreducible representations,  $H_1, H_2H_3$ , and  $H_4$ , which are two-, four- and six-dimensional, respectively. In particular,  $H_1$  and  $H_2H_3$  are realized as the lowest modes at the  $H$  point in the BPI and DG photonic crystals,

respectively, as summarized in Table 2. We find that  $\prod_i \frac{\xi_i(H)}{\zeta_i^+(H)} = 1$  for all the three possibilities,

by direct calculation from Table S4 in Supplemental Document. Second, the  $N$  point has two possible physically irreducible representations,  $N_1$  and  $N_2$ . Both of them are two-dimensional, consisting of one odd-parity and one even-parity modes. Thus, both irreps contribute to the product in Eq. (S4) by a factor  $\prod_{i \in N_a} \xi_i(N) = -1$  ( $a = 1, 2$ ). Therefore, the total contribution from the  $N$  point is  $(-1)^{n/2}$ , where  $n$  is the number of bands below the gap considered. Third, the  $\Gamma$  point allows ten irreps,  $\Gamma_{a\pm}$  ( $a = 1, \dots, 5$ ), and all of them have a product equal to  $\prod_i \zeta_i^+(\Gamma) = 1$ . Nonetheless, we need to note that the eigenmodes with  $\omega = 0$  at the  $\Gamma$  point are special in any photonic crystals. Because of the transversality condition of the electromagnetic wave, the eigenmodes with  $\omega = 0$  at the  $\Gamma$  point do not follow either of the ten irreps shown above, and therefore we need to calculate on such modes separately. From the previous subsection, because the two eigenmodes at  $\mathbf{k} = (0, k_y, 0)$  are two linearly polarized modes represented by  $\psi_x(0, k_y, 0) = \hat{x}e^{ik_y y}$  and  $\psi_z(0, k_y, 0) = \hat{z}e^{ik_y y}$ , we can construct eigenmodes in the  $g_+$  sector as  $\psi_x(0, k_y, 0) + \psi_x(0, -k_y, 0)$  and  $\psi_z(0, k_y, 0) + \psi_z(0, -k_y, 0)$ . Both of them have a  $C_{2y}$  eigenvalue equal to  $-1$ , and their product is  $+1$ , which contributes trivially to the product in Eq. (S4). To summarize, the glide- $Z_2$  invariant  $\nu$  for **230** is calculated as

$$(-1)^{\nu} = (-1)^{n/2} \rightarrow \nu = n/2 \pmod{2}. \quad (\text{S5})$$

It means that when the number of bands  $n$  below the gap is  $n = 4m+2$  ( $m$ : integer), the photonic crystal is topologically nontrivial, and when it is  $n = 4m$  ( $m$ : integer), it is topologically trivial, provided the gap is open everywhere in the Brillouin zone. We note the above results remains true for **206**, since the irreps at  $P$  points are identical to that of its supergroup **230**.

On the other hand, at the  $P$  point, there are two possible physically irreps under the TRS,  $P_1P_2$  and  $P_3$ , both of which are four-dimensional. Therefore, when  $n = 4m + 2$  (i.e.  $\nu = 1$ ), there is no gap at the  $P$  point when the TRS is preserved. Therefore, we need to open a gap at  $P$  by breaking TRS to make it topologically nontrivial. On the other hand, when  $n = 4m$  (i.e.  $\nu = 0$ ), the  $P$  point is gapped. Here, the  $P_1P_2$  and  $P_3$  irreps support the doubly degenerate Dirac point, and the generalized Dirac point, respectively, and in both cases, quad-helicoid surface states are realized on the (001) surface, without an anticrossing between two helicoids, thanks to the combination of the two glides and the time-reversal symmetries [10, 11], and another  $Z_2$  topological invariant could be defined to represent nontrivial winding of the helicoid surface states. Let us call it the helicoid- $Z_2$  invariant and how the helicoid- $Z_2$  and glide- $Z_2$  are mutually related is an open question.

We note that from Eq. (S4), the irreps at the  $P$  point in **230** do not contribute to the glide- $Z_2$  invariant. Thus, while this topological phase is realized by opening the band gap between the second and third bands at the  $P$  points when the photonic crystal has magnetization, this bandgap opening does not lead to topological band inversion. It is similar to the  $K$  point in the Kane-Mele model of Eq. (S1) with inversion symmetry.

Thus far, we have understood how to make nontrivial glide- $Z_2$  topological invariant in Eq. (7). To make the photonic crystal to have topological surface states, it is important how we break the TRS, i.e. how we introduce magnetization into dielectrics. Here we introduce two types of magnetizations, classified in terms of magnetic space groups (MSGs), and we call these types I and II. The type I is the MSG **142.565**, where the numberings of the MSG are summarized in the Bilbao Crystallographic Server [12]. It corresponds to the BPI photonic crystal with the two dielectric rods (red and yellow in Fig. 1 in the main text) having  $+z$  magnetization, and the other two (blue and green in Fig. 1 in the main text) having  $-z$  magnetization, as employed in Ref. [1]. The type II is the MSG **142.567**, corresponding to the DG photonic crystal with the uniform magnetization along the  $+z$  direction employed in Ref. [13]. From Eq. (S5), the photonic crystal is in the topological phase, if a gap is open between the second and the third lowest bands. We need to check whether the photonic crystal really opens a gap between the bands 2 and 3 when the TRS is broken. We find that in the type I the photonic crystal opens a gap everywhere in  $k$ -space, while in the type II, the photonic crystal does not open a gap. This is explained in terms of the minimal band connectivity  $M$  in photonic crystals. This notion of minimal band connectivity  $M$  for a nonmagnetic photonic crystal has been introduced in Ref. [14]. Here we extend the theory to magnetic photonic crystals. The minimal band connectivity  $M$  is defined as a minimum number of bands  $M$ , such that the gap can open everywhere in the Brillouin zone between the  $M$ th and  $(M+1)$ th bands. Because the two lowest bands in any photonic crystals approaches  $\omega = 0$  when  $\mathbf{k}$  approaches zero, the minimal band connectivity should be  $M \geq 2$ . We can show that the values of  $M$  is  $M = 2$  in type I (MSG **142.565**) and  $M \geq 4$  in type II (MSG **142.567**); it means that the gap between the second and third lowest bands can be open in type I, but not in type II.

### 3. TIGHT-BINDING MODEL FOR GLIDE- $Z_2$ TOPOLOGICAL PHASE WITH HINGE STATES

In the main text, we mention that in the presence of inversion symmetry, the glide- $Z_2$  topological phase is equivalent to a higher-order topological insulator phase, as proposed in Refs. [5-8]. In this appendix, to demonstrate this equivalence, we numerically confirm existence of the hinge states in the glide- $Z_2$  topological phase in a simple tight-binding model. To this end, let us consider the following eight-band tight-binding model. The unit cell consists of four lattice sites A1  $(0, \frac{1}{4}, 0)$ , A2  $(0, \frac{3}{4}, 0)$ , B1  $(0, \frac{1}{4}, \frac{1}{2})$ , and B2  $(0, \frac{3}{4}, \frac{1}{2})$ , and the primitive translation vectors are  $(1, 0, 0)$ ,  $(0, 1, 0)$  and  $(0, 0, 1)$ , where the lattice constants are set to be unity (see Fig. S3(a)). We take the model to be in the space group No. 50 ( $P4_2/m$ ), and the four sites are in the Wyckoff positions  $4i$ . The model consists of two kinds of layers along the  $xy$  plane, alternately stacked along the  $z$  direction, and each layer is a two-dimensional Chern insulator. One layer is a Chern insulator layer with the Chern number  $C = +1$  on  $z = n$ ,  $n \in \mathbf{Z}$  consisting of A1 and A2 sublattices, and the other is a Chern insulator layer with the Chern number  $C = -1$  on  $z = n + \frac{1}{2}$ ,  $n \in \mathbf{Z}$  consisting of B1 and B2 sublattices. Let  $H^A$  and  $H^B$  denote the Hamiltonians for the former layers and the latter layers, respectively. Within this symmetry, we also introduce interlayer hoppings  $H^{AB}$ . The Hamiltonian is written as

$$H = H^A + H^B + H^{AB}, \quad (\text{S6})$$

$$H^A = \sum_n \sum_{r \in (\mathbf{Z}, \mathbf{Z}/2 - 1/4)} \left[ m \psi_{A,r,n}^\dagger \sigma_z \psi_{A,r,n} + \left( \psi_{A,r+\hat{x},n}^\dagger \frac{\sigma_z + i\sigma_x}{2} \psi_{A,r,n} + \text{h.c.} \right) \right. \\ \left. + \left( \psi_{A,r+y/2,n}^\dagger \frac{\sigma_z + i\sigma_y}{2} \psi_{A,r,n} + \text{h.c.} \right) \right], \quad (\text{S7})$$

$$(\text{S8})$$

$$\begin{aligned}
H^B = \sum_n \sum_{\mathbf{r}=(\mathbf{Z}, \mathbf{Z}/2-1/4)} & [m\psi_{B,\mathbf{r},n}^\dagger \sigma_z \psi_{B,\mathbf{r},n} + \left( \psi_{B,\mathbf{r}+\hat{y}/2,n}^\dagger \frac{\sigma_z - i\sigma_y}{2} \psi_{B,\mathbf{r},n} + \text{h.c.} \right) \\
& + \left( \psi_{B,\mathbf{r}+\hat{x},n}^\dagger \frac{\sigma_z + i\sigma_x}{2} \psi_{B,\mathbf{r},n} + \text{h.c.} \right)], \\
H^{AB} = \frac{1}{2} \sum_n & \left[ \sum_{\mathbf{r}=(\mathbf{Z}, \mathbf{Z}+1/4)} \psi_{A,\mathbf{r},n}^\dagger \psi_{B,\mathbf{r},n} + \sum_{\mathbf{r}=(\mathbf{Z}, \mathbf{Z}-1/4)} \psi_{A,\mathbf{r},n+1}^\dagger \psi_{B,\mathbf{r},n} + \text{h.c.} \right] \quad (\text{S9})
\end{aligned}$$

where  $\mathbf{r}$  runs over the lattice sites within the  $xy$  plane,  $\mathbf{r} = (r_1, r_2)$ ,  $r_1 \in \mathbf{Z}$ ,  $r_2 \in \mathbf{Z} \pm \frac{1}{4}$ ,  $\sigma_\alpha$  ( $\alpha = x, y, z$ ) are the Pauli matrices, and  $\psi_{A,\mathbf{r},n}$  ( $\psi_{B,\mathbf{r},n}$ ) is an annihilation operator at the lattice site at  $(\mathbf{r}, n)$  in the sublattice A (at  $(\mathbf{r}, n + \frac{1}{2})$  in the sublattice B). When the interlayer term  $H^{AB}$  is absent, it is exactly the model of the layer construction called (010; 0), which is known to show the glide- $Z_2$  topological phase in some parameter range. As we show later, this model preserves the glide symmetry and inversion symmetry. The surface state originating from the chiral edge states of the Chern-insulator layers always appear. We then add the term  $H^{AB}$  to see whether hinge states of the higher-order topological insulating phase appear.

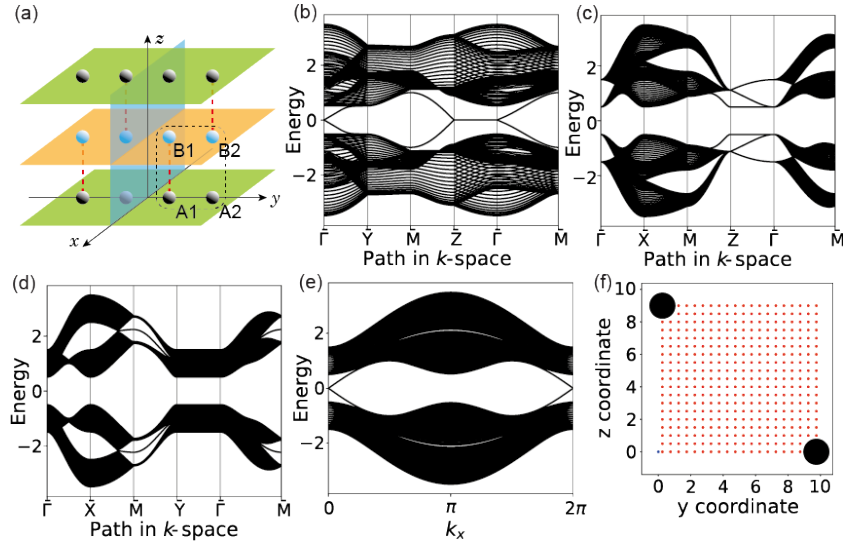

Fig. S3. (a) Schematic figure of our model showing a glide- $Z_2$  topological phase with four sites in the unit cell marked by the black dotted line. The model is manifestly invariant under glide symmetry and inversion symmetry. (b)-(d) Band structures for slabs with (b) the (100) surfaces, (c) the (010) surfaces, and (d) the (001) surfaces. The thickness of the slab is  $n=20$ . In (b), the gapless surface states exist on the (100) surface which preserves glide symmetry. On the other hand, the surface states are gapped on (c) the (010) surface and (d) the (001) surface breaking glide symmetry. The high-symmetry points are given as  $\bar{\Gamma} = (0, 0)$ ,  $\bar{M} = (\pi, \pi)$  on the (100), (010), and (001) surfaces,  $\bar{Y} = (\pi, 0)$ ,  $\bar{Z} = (0, \pi)$  on the (100) surface,  $\bar{X} = (\pi, 0)$ ,  $\bar{Z} = (0, \pi)$  on the (010) surface, and  $\bar{X} = (\pi, 0)$ ,  $\bar{Y} = (0, \pi)$  on the (001) surface. (e) The gapless band structure for the rod configuration. The rod is finite along the  $y$  and  $z$  direction with the sizes of the system along the two directions equal to  $n=10$ , and is periodic along the  $x$  direction. It is gapless, with the gapless states lying on hinges. (f) Density plot of the wavefunctions of the gapless states. They are localized on hinges of the rod.

The Hamiltonian  $H$  shows the glide- $Z_2$  topological phase if  $-1.5 < m < -0.5$  and  $0.5 < m < 1.5$ , the Weyl semimetal phase if  $1.5 < |m| < 2.5$  and  $|m| < 0.5$ , and a trivial phase if  $2.5 < |m|$ . Let us focus on the glide- $Z_2$  topological phase at  $m = -1$ . Figures S3(b)-(d) are band structures of a slab with (b) the (100) surface, (c) the (010) surface, and (d) the (001) surface. The gapless surface states emerge on the (100) surface preserving the glide symmetry [Fig. S3(b)] while the band structures are gapped on the (010) surface [Fig. S3(c)] and the (001) surface [Fig. S3(d)].

Here we comment on the flat dispersion of the gapless surface states along the  $\bar{Z} - \bar{\Gamma} - \bar{Z}$  in Fig. S3(b). It has been known that the topologically nontrivial phase with the glide symmetry has a single surface Dirac cone either along  $\bar{Z} - \bar{\Gamma} - \bar{Z}$  or  $\bar{M} - \bar{Y} - \bar{M}$  [3, 4]. We first note that by additional inversion  $I = \{I|0\}$  and glide  $G_z = \{M_z|\frac{1}{2}\hat{y}\}$  symmetries of the model, the topological surface Dirac cone is expected at either of the high-symmetry points at  $\bar{Z}$ ,  $\bar{\Gamma}$ ,  $\bar{Y}$ , or  $\bar{M}$ . Although the flat dispersion in Fig. S3 may look different from the expected Dirac cone, we here explain that the flat dispersion along the  $\bar{Z} - \bar{\Gamma} - \bar{Z}$  line is indeed a special case of the single Dirac cone at  $\bar{Z}$ , and that this flat dispersion is caused by other additional symmetries in this model. First, this model preserves particle-hole symmetry represented by an operator  $U = \sigma_y \tau_y \text{diag}(1, \exp(-ik_y))_\rho$ , where  $\tau$  and  $\rho$  are matrices acting on the sublattice space spanned by four sublattice sites  $(\tau_z, \rho_z) = (+, +), (+, -), (-, +), (-, -)$  for the A1, A2, B1 and B2 sublattices respectively. Then the Hamiltonian  $H(k)$  preserves the particle-hole symmetry;  $U(k)H(k)U(k)^{-1} = -H(k)^*$ , meaning that the spectrum is symmetric with respect to  $E = 0$ , and the Dirac point for the topological surface Dirac cone appears at  $E = 0$ . In the slab calculation, such a Dirac point at  $E = 0$  appears at the  $\bar{Z}$  point, and it consists of two states per each surface, with glide eigenvalues  $g_y = +i$  and  $g_y = -i$ . Next, we consider how these degenerate states evolve along the  $\bar{Z} - \bar{\Gamma}$  line. On this line, the Hamiltonian has an additional symmetry, represented by  $Q = \rho_y$ , commuting with the Hamiltonian. Therefore, along the  $\bar{Z} - \bar{\Gamma}$  line, the glide symmetry  $G_y = \{M_y|\frac{1}{2}\hat{z}\}$  represented by an operator

$$G_y = \begin{pmatrix} & \exp(-ik_z) \\ 1 & \end{pmatrix}_\tau \rho_x \quad (\text{S10})$$

and the  $Q$  symmetry are both preserved, and they anticommute. Therefore, along this  $\bar{Z} - \bar{\Gamma}$  line the two states with  $g_y = \exp(-ik_z/2)$  and  $g_y = -\exp(-ik_z/2)$  remain degenerate, and they remain fixed at  $E = 0$  due to the particle-hole symmetry. Thus, to summarize, the flat surface dispersion on the  $\bar{Z} - \bar{\Gamma}$  line can be regarded as a single Dirac-cone topological surface states due to the glide symmetry, and this flattening of the dispersion is caused by the additional symmetry represented by the  $Q$  operator on the  $k_y = 0$ , the glide  $G_y$  symmetry and the particle-hole symmetry.

As we wrote in Sec. 5 in the main text, the glide- $Z_2$  topological crystalline insulator is identically the higher-order topological insulator in the presence of inversion symmetry. This comes from the relation  $v = z_4/2 \pmod{2}$  in which  $z_4$  is the  $Z_4$  topological invariant defined modulo 4 for centrosymmetric systems [7,8]. To see the hinge states characteristic of the higher-order topological insulator phase, the topological surface states should be absent, because otherwise the hinge states are hidden behind. To this end, we consider rod configuration with (010) and (001) surfaces, which is periodic along the  $x$  direction. We then show that the band structure for the rod geometry exhibits the gapless states depicted in Fig. S3(e). The wavefunctions of the gapless states are strongly localized on hinges of the rod, as is seen in the density of the wavefunctions of the gapless states in Fig. S3(f). This results indeed show that the glide- $Z_2$  topological crystalline insulator is identically the higher-order topological insulator in the presence of inversion symmetry, as expected.

#### 4. SUMMARY OF TABLES USED FOR THE SYMMETRY ANALYSIS

Here we summarize useful information for the calculations in the main text. Table S1 shows decompositions of the plane-wave electromagnetic waves in vacuum into irreps in **230** for the lowest several bands at the high-symmetry points in the Brillouin zone of the BCC lattice, used in Sec. 3 in the main text.

In the decomposition into irreps in making Table S1, we use the character table of irreducible representations at high-symmetry points H and N in Table S3, and we summarize some of their matrix forms used in the main text in Table S4. We show the compatibility relations between the P point and the H point via  $\Lambda$  in Table S2 in **230** [9]. It shows the relationships between the irreps at P point and those at H point and along the  $C_3$ -symmetric  $\Lambda$  line. This compatibility relations are used for the analysis of band connectivities in Sec. 3.3. When the time-reversal symmetry is considered, the irreps in the curly bracket are degenerate, forming a physically irrep. The full information is summarized in the database in Ref. [9]. The Wyckoff positions in **230** used throughout the paper are shown in Table S5 [14]. The multiplicities and the Wyckoff letters are shown in the first column, the site symmetry is shown in the second column, and the coordinates with two sets  $(0, 0, 0)^+$  and  $(\frac{1}{2}, \frac{1}{2}, \frac{1}{2})^+$  are given in the rest of Table S5 [14].

**Table S1. Summary of the characters for the representations of the lowest bands at high symmetry wavevectors and their decomposition into irreducible representations at the 8 smallest wavevectors in vacuum with a frequency  $\Omega_0$  where  $b = 2\pi/a$  with the lattice constant  $a$  in **230** with the TRS. Here  $C_2 = \{2_{001}|0 \frac{1}{2} 0\}$ ,  $C_3 = \{3^+_{111}|000\}$ ,  $C_4 = \{4^+_{111}|\frac{1}{4} \frac{3}{4} \frac{1}{4}\}$ ,  $C'_2 = \{2_{110}|\frac{3}{4} \frac{1}{4} \frac{1}{4}\}$ , and  $I = \{1|000\}$ .  $3C_2$ ,  $8C_3$ ,  $6C_4$  and  $6C'_2$  represent the conjugacy classes of the respective symmetry operation. The numbers in the parentheses represent the dimensions of the irreps**

| $R$            | $\Omega_0$             | $E$ | $3C_2$ | $8C_3$ | $6C_4$ | $6C'_2$ | $I$ | $3IC_2$ | $8IC_3$ | $6IC_4$ | $6IC'_2$ | Irreps                        |
|----------------|------------------------|-----|--------|--------|--------|---------|-----|---------|---------|---------|----------|-------------------------------|
| $\Gamma^{(1)}$ | $\sqrt{2}b$            | 24  | 0      | 0      | 0      | -24     | 0   | 0       | 0       | 0       | 0        |                               |
| $H^{(0)}$      | $b$                    | 12  | -4     | 0      | 0      | 0       | 0   | 0       | 0       | 0       | 0        | $H_1(2) + H_2H_3(4) + H_4(6)$ |
| $H^{(1)}$      | $\sqrt{3}b$            | 16  | 0      | -2     | 0      | 0       | 0   | 0       | 0       | 0       | 0        | $H_2H_3(4) + 2H_4(6)$         |
| $N^{(0)}$      | $\frac{\sqrt{2}}{2}b$  | 4   | 0      | -      | -      | 4       | 0   | 0       | -       | -       | 0        | $2N_1(2)$                     |
| $N^{(1)}$      | $\frac{\sqrt{6}}{2}b$  | 8   | 0      | -      | -      | 0       | 0   | 0       | -       | -       | 0        | $2N_1(2) + 2N_2(2)$           |
| $N^{(2)}$      | $\frac{\sqrt{10}}{2}b$ | 8   | 0      | -      | -      | 0       | 0   | 0       | -       | -       | 0        | $2N_1(2) + 2N_2(2)$           |
| $P^{(0)}$      | $\frac{\sqrt{2}}{2}b$  | 8   | 0      | -1     | -      | -       | -   | -       | -       | 0       | 0        | $P_1P_2(4) + P_3(4)$          |
| $P^{(1)}$      | $\frac{\sqrt{11}}{2}b$ | 24  | 0      | 0      | -      | -       | -   | -       | -       | 0       | 0        | $2P_1P_2(4) + 4P_3(4)$        |

**Table S2. Compatibility relations with time-reversal symmetry between the P point and the H point via the  $\Lambda$  line, which is along the  $C_3$  invariant axis. The curly bracket  $\{ \}$  represents physically irreducible representations, which are degenerate when the TRS is present. The full information is summarized in Ref. [9].**

| k-vector | Compatibility relations                                                                                                    | k-vector  | Compatibility relations                                                                                                                                                             | k-vector |
|----------|----------------------------------------------------------------------------------------------------------------------------|-----------|-------------------------------------------------------------------------------------------------------------------------------------------------------------------------------------|----------|
| $P$      | $\{P_1(2) P_2(2)\} \rightarrow 2\Lambda_3(2)$<br>$P_3(4) \rightarrow \Lambda_1(1) \oplus \Lambda_2(1) \oplus \Lambda_3(2)$ | $\Lambda$ | $H_1(2) \rightarrow \Lambda_1(1) \oplus \Lambda_2(1)$<br>$\{H_2(2)H_3(2)\} \rightarrow 2\Lambda_3(2)$<br>$H_4(6) \rightarrow \Lambda_1(1) \oplus \Lambda_2(1) \oplus 2\Lambda_3(2)$ | $H$      |

**Table S3. Summary of characters of irreducible representations at high-symmetry points H and N adopted from Ref. [9].**

|                                                       | $H_1$ | $H_2$ | $H_3$ | $H_4$ | $N_1$ | $N_2$ |                                                          | $H_1$ | $H_2$        | $H_3$        | $H_4$ | $N_1$ | $N_2$ |
|-------------------------------------------------------|-------|-------|-------|-------|-------|-------|----------------------------------------------------------|-------|--------------|--------------|-------|-------|-------|
| $\{1 t_1 t_2 t_3\}$                                   | 2     | 2     | 2     | 6     | 2     | 2     | $\{\bar{1} 000\}$                                        | 0     | 0            | 0            | 0     | 0     | 0     |
| $\{2_{001} 0_{\frac{1}{2}}0\}$                        | -2    | -2    | -2    | 2     | 0     | 0     | $\{m_{001} 0_{\frac{1}{2}}0\}$                           | 0     | 0            | 0            | 0     | 0     | 0     |
| $\{2_{010} \frac{1}{2}00\}$                           | -2    | -2    | -2    | 2     |       |       | $\{m_{010} \frac{1}{2}00\}$                              | 0     | 0            | 0            | 0     |       |       |
| $\{2_{100} 00\frac{1}{2}\}$                           | -2    | -2    | -2    | 2     |       |       | $\{m_{100} 00\frac{1}{2}\}$                              | 0     | 0            | 0            | 0     |       |       |
| $\{3^+_{111} 000\}$                                   | 2     | -1    | -1    | 0     |       |       | $\{\bar{3}^+_{111} 000\}$                                | 0     | $-\sqrt{3}i$ | $\sqrt{3}i$  | 0     |       |       |
| $\{3^+_{\bar{1}\bar{1}\bar{1}} 00\frac{1}{2}\}$       | -2    | 1     | 1     | 0     |       |       | $\{\bar{3}^+_{\bar{1}\bar{1}\bar{1}} 00\frac{1}{2}\}$    | 0     | $\sqrt{3}i$  | $-\sqrt{3}i$ | 0     |       |       |
| $\{3^+_{1\bar{1}\bar{1}} 0_{\frac{1}{2}}0\}$          | -2    | 1     | 1     | 0     |       |       | $\{\bar{3}^+_{1\bar{1}\bar{1}} 0_{\frac{1}{2}}0\}$       | 0     | $\sqrt{3}i$  | $-\sqrt{3}i$ | 0     |       |       |
| $\{3^+_{\bar{1}\bar{1}1} \frac{1}{2}00\}$             | -2    | 1     | 1     | 0     |       |       | $\{\bar{3}^+_{\bar{1}\bar{1}1} \frac{1}{2}00\}$          | 0     | $\sqrt{3}i$  | $-\sqrt{3}i$ | 0     |       |       |
| $\{3^-_{111} 000\}$                                   | 2     | -1    | -1    | 0     |       |       | $\{\bar{3}^-_{111} 000\}$                                | 0     | $\sqrt{3}i$  | $-\sqrt{3}i$ | 0     |       |       |
| $\{3^-_{1\bar{1}\bar{1}} \frac{1}{2}00\}$             | -2    | 1     | 1     | 0     |       |       | $\{\bar{3}^-_{1\bar{1}\bar{1}} \frac{1}{2}00\}$          | 0     | $-\sqrt{3}i$ | $\sqrt{3}i$  | 0     |       |       |
| $\{3^-_{\bar{1}\bar{1}1} 00\frac{1}{2}\}$             | -2    | 1     | 1     | 0     |       |       | $\{\bar{3}^-_{\bar{1}\bar{1}1} 00\frac{1}{2}\}$          | 0     | $-\sqrt{3}i$ | $\sqrt{3}i$  | 0     |       |       |
| $\{3^-_{\bar{1}\bar{1}\bar{1}} 0_{\frac{1}{2}}0\}$    | -2    | 1     | 1     | 0     |       |       | $\{\bar{3}^-_{\bar{1}\bar{1}\bar{1}} 0_{\frac{1}{2}}0\}$ | 0     | $-\sqrt{3}i$ | $\sqrt{3}i$  | 0     |       |       |
| $\{2_{110} \frac{3}{4}\frac{1}{4}\frac{1}{4}\}$       | 0     | 0     | 0     | 0     | 2     | -1    | $\{m_{110} \frac{3}{4}\frac{1}{4}\frac{1}{4}\}$          | 0     | 0            | 0            | 0     | 0     | 0     |
| $\{2_{1\bar{1}0} \frac{1}{4}\frac{1}{4}\frac{1}{4}\}$ | 0     | 0     | 0     | 0     | 0     | 0     | $\{m_{1\bar{1}0} \frac{1}{4}\frac{1}{4}\frac{1}{4}\}$    | 0     | 0            | 0            | 0     | 0     | 0     |
| $\{4^-_{001} \frac{1}{4}\frac{1}{4}\frac{3}{4}\}$     | 0     | 0     | 0     | 0     |       |       | $\{\bar{4}^-_{001} \frac{1}{4}\frac{1}{4}\frac{3}{4}\}$  | 0     | 0            | 0            | 0     |       |       |
| $\{4^+_{001} \frac{1}{4}\frac{3}{4}\frac{1}{4}\}$     | 0     | 0     | 0     | 0     |       |       | $\{\bar{4}^+_{001} \frac{1}{4}\frac{3}{4}\frac{1}{4}\}$  | 0     | 0            | 0            | 0     |       |       |
| $\{4^-_{100} \frac{3}{4}\frac{1}{4}\frac{1}{4}\}$     | 0     | 0     | 0     | 0     |       |       | $\{\bar{4}^-_{100} \frac{3}{4}\frac{1}{4}\frac{1}{4}\}$  | 0     | 0            | 0            | 0     |       |       |
| $\{2_{011} \frac{1}{4}\frac{3}{4}\frac{1}{4}\}$       | 0     | 0     | 0     | 0     |       |       | $\{m_{011} \frac{1}{4}\frac{3}{4}\frac{1}{4}\}$          | 0     | 0            | 0            | 0     |       |       |
| $\{2_{01\bar{1}} \frac{1}{4}\frac{1}{4}\frac{1}{4}\}$ | 0     | 0     | 0     | 0     |       |       | $\{m_{01\bar{1}} \frac{1}{4}\frac{1}{4}\frac{1}{4}\}$    | 0     | 0            | 0            | 0     |       |       |
| $\{4^+_{100} \frac{1}{4}\frac{1}{4}\frac{3}{4}\}$     | 0     | 0     | 0     | 0     |       |       | $\{\bar{4}^+_{100} \frac{1}{4}\frac{1}{4}\frac{3}{4}\}$  | 0     | 0            | 0            | 0     |       |       |
| $\{4^+_{010} \frac{3}{4}\frac{1}{4}\frac{1}{4}\}$     | 0     | 0     | 0     | 0     |       |       | $\{\bar{4}^+_{010} \frac{3}{4}\frac{1}{4}\frac{1}{4}\}$  | 0     | 0            | 0            | 0     |       |       |
| $\{2_{101} \frac{1}{4}\frac{1}{4}\frac{3}{4}\}$       | 0     | 0     | 0     | 0     |       |       | $\{m_{101} \frac{1}{4}\frac{1}{4}\frac{3}{4}\}$          | 0     | 0            | 0            | 0     |       |       |
| $\{4^-_{010} \frac{1}{4}\frac{3}{4}\frac{1}{4}\}$     | 0     | 0     | 0     | 0     |       |       | $\{\bar{4}^-_{010} \frac{1}{4}\frac{3}{4}\frac{1}{4}\}$  | 0     | 0            | 0            | 0     |       |       |
| $\{2_{\bar{1}01} \frac{1}{4}\frac{1}{4}\frac{1}{4}\}$ | 0     | 0     | 0     | 0     |       |       | $\{m_{\bar{1}01} \frac{1}{4}\frac{1}{4}\frac{1}{4}\}$    | 0     | 0            | 0            | 0     |       |       |

**Table S4. Summary of matrices for the irreducible representations at high-symmetry points  $\Gamma = (0, 0, 0)$ ,  $H = (\frac{1}{2}, 0, \frac{1}{2})$  and  $N = (\frac{1}{2}, \frac{1}{2}, \frac{1}{2})$  adopted from Ref. [9]. We show the matrices for the inversion, twofold rotation and glide reflections only, which we use for a calculation of the glide- $Z_2$  invariant in the main text. Note that the convention for the symmetry operations are a bit different from that used in the main text, but this difference does not affect the calculation of the glide- $Z_2$  invariant.**

|              | $\{\bar{1} 000\}$                                          | $\{2_{010} \frac{1}{2}^{00}\}$                            | $\{m_{010} \frac{1}{2}^{00}\}$                            |
|--------------|------------------------------------------------------------|-----------------------------------------------------------|-----------------------------------------------------------|
| $\Gamma_1^+$ | 1                                                          | 1                                                         | 1                                                         |
| $\Gamma_1^-$ | -1                                                         | 1                                                         | -1                                                        |
| $\Gamma_2^+$ | 1                                                          | 1                                                         | 1                                                         |
| $\Gamma_2^-$ | -1                                                         | 1                                                         | -1                                                        |
| $\Gamma_3^+$ | $\begin{pmatrix} 1 & \\ & 1 \end{pmatrix}$                 | $\begin{pmatrix} 1 & \\ & 1 \end{pmatrix}$                | $\begin{pmatrix} 1 & \\ & 1 \end{pmatrix}$                |
| $\Gamma_3^-$ | $\begin{pmatrix} -1 & \\ & -1 \end{pmatrix}$               | $\begin{pmatrix} 1 & \\ & 1 \end{pmatrix}$                | $\begin{pmatrix} -1 & \\ & -1 \end{pmatrix}$              |
| $\Gamma_4^+$ | $\begin{pmatrix} 1 & & \\ & 1 & \\ & & 1 \end{pmatrix}$    | $\begin{pmatrix} -1 & & \\ & -1 & \\ & & 1 \end{pmatrix}$ | $\begin{pmatrix} -1 & & \\ & -1 & \\ & & 1 \end{pmatrix}$ |
| $\Gamma_4^-$ | $\begin{pmatrix} -1 & & \\ & -1 & \\ & & -1 \end{pmatrix}$ | $\begin{pmatrix} -1 & & \\ & -1 & \\ & & 1 \end{pmatrix}$ | $\begin{pmatrix} 1 & & \\ & 1 & \\ & & -1 \end{pmatrix}$  |
| $\Gamma_5^+$ | $\begin{pmatrix} 1 & & \\ & 1 & \\ & & 1 \end{pmatrix}$    | $\begin{pmatrix} -1 & & \\ & -1 & \\ & & 1 \end{pmatrix}$ | $\begin{pmatrix} -1 & & \\ & -1 & \\ & & 1 \end{pmatrix}$ |
| $\Gamma_5^-$ | $\begin{pmatrix} -1 & & \\ & -1 & \\ & & -1 \end{pmatrix}$ | $\begin{pmatrix} -1 & & \\ & -1 & \\ & & 1 \end{pmatrix}$ | $\begin{pmatrix} 1 & & \\ & 1 & \\ & & -1 \end{pmatrix}$  |
| $N_1$        | $\begin{pmatrix} 1 & \\ & -1 \end{pmatrix}$                | $\begin{pmatrix} & -1 \\ -1 & \end{pmatrix}$              | $\begin{pmatrix} & 1 \\ -1 & \end{pmatrix}$               |
| $N_2$        | $\begin{pmatrix} 1 & \\ & -1 \end{pmatrix}$                | $\begin{pmatrix} & 1 \\ 1 & \end{pmatrix}$                | $\begin{pmatrix} & -1 \\ 1 & \end{pmatrix}$               |
| $H_1$        | $\begin{pmatrix} 1 & \\ & -1 \end{pmatrix}$                | $\begin{pmatrix} -1 & \\ & -1 \end{pmatrix}$              | $\begin{pmatrix} -1 & \\ & 1 \end{pmatrix}$               |
| $H_2$        | $\begin{pmatrix} 1 & \\ & -1 \end{pmatrix}$                | $\begin{pmatrix} -1 & \\ & -1 \end{pmatrix}$              | $\begin{pmatrix} -1 & \\ & 1 \end{pmatrix}$               |
| $H_3$        | $\begin{pmatrix} 1 & \\ & -1 \end{pmatrix}$                | $\begin{pmatrix} -1 & \\ & -1 \end{pmatrix}$              | $\begin{pmatrix} -1 & \\ & 1 \end{pmatrix}$               |
| $H_4$        | diag(1, 1, 1, -1, -1, -1)                                  | diag(1, -1, 1, -1, 1, 1)                                  | diag(1, -1, 1, 1, -1, -1)                                 |

**Table S5. Summary of Wyckoff positions in 230 except for the most general one 96h. The first column denotes the multiplicity and the Wyckoff letter, the second column denotes site symmetry, and the coordinates with two sets  $(0, 0, 0)+$  and  $(\frac{1}{2}, \frac{1}{2}, \frac{1}{2})+$ . Asymmetric unit is given by  $-\frac{1}{8} \leq x \leq \frac{1}{8}; -\frac{1}{8} \leq y \leq \frac{1}{8}; 0 \leq z \leq \frac{1}{4}; \max(x, -x, y, -y) \leq z$  adopted from Ref. [14].**

|     |       |                                                                 |                                                                       |                                                                 |                                                                 |
|-----|-------|-----------------------------------------------------------------|-----------------------------------------------------------------------|-----------------------------------------------------------------|-----------------------------------------------------------------|
| 48g | ..2   | $\frac{1}{8}, y, \bar{y} + \frac{1}{4}$                         | $\frac{3}{8}, \bar{y}, \bar{y} + \frac{3}{4}$                         | $\frac{7}{8}, y + \frac{1}{2}, y + \frac{1}{4}$                 | $\frac{5}{8}, \bar{y} + \frac{1}{2}, y + \frac{3}{4}$           |
|     |       | $\bar{y} + \frac{1}{4}, \frac{1}{8}, y$                         | $\bar{y} + \frac{3}{4}, \frac{3}{8}, \bar{y}$                         | $y + \frac{1}{4}, \frac{7}{8}, y + \frac{1}{2}$                 | $y + \frac{3}{4}, \frac{5}{8}, \bar{y} + \frac{1}{2}$           |
|     |       | $y, \bar{y} + \frac{1}{4}, \frac{1}{8}$                         | $\bar{y}, \bar{y} + \frac{3}{4}, \frac{7}{8}$                         | $y + \frac{1}{2}, y + \frac{1}{4}, \frac{7}{8}$                 | $\bar{y} + \frac{1}{2}, y + \frac{3}{4}, \frac{5}{8}$           |
|     |       | $\frac{7}{8}, \bar{y}, y + \frac{3}{4}$                         | $\frac{5}{8}, y, y + \frac{1}{4}$                                     | $\frac{1}{8}, \bar{y} + \frac{1}{2}, \bar{y} + \frac{3}{4}$     | $\frac{3}{8}, y + \frac{1}{2}, \bar{y} + \frac{1}{4}$           |
|     |       | $y + \frac{3}{4}, \frac{7}{8}, \bar{y}$                         | $y + \frac{1}{4}, \frac{5}{8}, y$                                     | $\bar{y} + \frac{3}{4}, \frac{1}{8}, \bar{y} + \frac{1}{2}$     | $\bar{y} + \frac{1}{4}, \frac{3}{8}, y + \frac{1}{2}$           |
|     |       | $\bar{y}, y + \frac{3}{4}, \frac{7}{8}$                         | $y, y + \frac{1}{4}, \frac{5}{8}$                                     | $\bar{y} + \frac{1}{2}, \bar{y} + \frac{3}{4}, \frac{1}{8}$     | $y + \frac{1}{2}, \bar{y} + \frac{1}{4}, \frac{3}{8}$           |
| 48f | 2..   | $x, 0, \frac{1}{4}$                                             | $\bar{x} + \frac{1}{2}, 0, \frac{3}{4}$                               | $\frac{1}{4}, x, 0$                                             | $\frac{3}{4}, \bar{x} + \frac{1}{2}, 0$                         |
|     |       | $0, \frac{1}{4}, x$                                             | $0, \frac{3}{4}, \bar{x} + \frac{1}{2}$                               | $\frac{3}{4}, x + \frac{1}{4}, 0$                               | $\frac{3}{4}, \bar{x} + \frac{3}{4}, \frac{1}{2}$               |
|     |       | $x + \frac{3}{4}, \frac{1}{4}, \frac{1}{4}$                     | $\bar{x} + \frac{1}{4}, 0, \frac{1}{4}$                               | $0, \frac{1}{4}, \bar{x} + \frac{1}{4}$                         | $\frac{1}{2}, \frac{1}{4}, x + \frac{3}{4}$                     |
|     |       | $\bar{x}, 0, \frac{3}{4}$                                       | $x + \frac{1}{2}, 0, \frac{1}{4}$                                     | $\frac{3}{4}, \bar{x}, 0$                                       | $\frac{1}{4}, x + \frac{1}{2}, 0$                               |
|     |       | $0, \frac{3}{4}, \bar{x}$                                       | $0, \frac{1}{4}, x + \frac{1}{2}$                                     | $\frac{1}{4}, \bar{x} + \frac{3}{4}, 0$                         | $\frac{1}{4}, x + \frac{1}{4}, \frac{1}{2}$                     |
|     |       | $\bar{x} + \frac{1}{4}, \frac{1}{4}, \frac{3}{4}$               | $x + \frac{3}{4}, 0, \frac{3}{4}$                                     | $0, \frac{3}{4}, x + \frac{3}{4}$                               | $\frac{1}{2}, \frac{3}{4}, \bar{x} + \frac{1}{4}$               |
| 32e | .3.   | $x, x, x$                                                       | $\bar{x} + \frac{1}{2}, \bar{x}, x + \frac{1}{2}$                     | $\bar{x}, x + \frac{1}{2}, \bar{x} + \frac{1}{2}$               | $x + \frac{1}{2}, \bar{x} + \frac{1}{2}, \bar{x}$               |
|     |       | $x + \frac{3}{4}, x + \frac{1}{4}, \bar{x} + \frac{1}{4}$       | $\bar{x} + \frac{3}{4}, \bar{x} + \frac{3}{4}, \bar{x} + \frac{3}{4}$ | $x + \frac{1}{4}, \bar{x} + \frac{1}{4}, x + \frac{3}{4}$       | $\bar{x} + \frac{1}{4}, x + \frac{3}{4}, x + \frac{1}{4}$       |
|     |       | $\bar{x}, \bar{x}, \bar{x}$                                     | $x + \frac{1}{2}, x, \bar{x} + \frac{1}{2}$                           | $x, \bar{x} + \frac{1}{2}, x + \frac{1}{2}$                     | $\bar{x} + \frac{1}{2}, x + \frac{1}{2}, x$                     |
|     |       | $\bar{x} + \frac{1}{4}, \bar{x} + \frac{3}{4}, x + \frac{3}{4}$ | $x + \frac{1}{4}, x + \frac{1}{4}, x + \frac{1}{4}$                   | $\bar{x} + \frac{3}{4}, x + \frac{3}{4}, \bar{x} + \frac{1}{4}$ | $x + \frac{3}{4}, \bar{x} + \frac{1}{4}, \bar{x} + \frac{3}{4}$ |
| 24d | 4..   | $\frac{3}{8}, 0, \frac{1}{4}$                                   | $\frac{1}{8}, 0, \frac{3}{4}$                                         | $\frac{1}{4}, \frac{3}{8}, 0$                                   | $\frac{3}{4}, \frac{1}{8}, 0$                                   |
|     |       | $\frac{3}{4}, \frac{5}{8}, 0$                                   | $\frac{3}{4}, \frac{3}{8}, \frac{1}{2}$                               | $\frac{1}{4}, \frac{1}{8}, 0$                                   | $\frac{1}{4}, \frac{7}{8}, 0$                                   |
| 24e | 2.2 2 | $\frac{1}{8}, 0, \frac{1}{4}$                                   | $\frac{3}{8}, 0, \frac{3}{4}$                                         | $\frac{1}{4}, \frac{1}{8}, 0$                                   | $\frac{3}{4}, \frac{3}{8}, 0$                                   |
|     |       | $\frac{7}{8}, 0, \frac{3}{4}$                                   | $\frac{5}{8}, 0, \frac{1}{4}$                                         | $\frac{3}{4}, \frac{7}{8}, 0$                                   | $\frac{1}{4}, \frac{5}{8}, 0$                                   |
| 16b | .32   | $\frac{1}{8}, \frac{1}{8}, \frac{1}{8}$                         | $\frac{3}{8}, \frac{7}{8}, \frac{5}{8}$                               | $\frac{7}{8}, \frac{5}{8}, \frac{3}{8}$                         | $\frac{5}{8}, \frac{3}{8}, \frac{7}{8}$                         |
| 16a | .3.   | $0, 0, 0$                                                       | $\frac{1}{2}, 0, \frac{1}{2}$                                         | $0, \frac{1}{2}, \frac{1}{2}$                                   | $\frac{1}{2}, \frac{1}{2}, 0$                                   |

## 5. MINIMAL BAND CONNECTIVITY FOR THE MSG 142.567

In this appendix we show that the minimal band connectivity  $M$  for the MSG **142.567** satisfies  $M \geq 4$ , which prohibits a common band gap throughout the Brillouin zone between the bands 2 and 3. We focus on the eigenvalues of the twofold rotation  $C_{2z} = \{2_{001}|0_2^1 0\}$  along the high symmetry line W  $(\pi/a, \pi/a, k_z)$ , which connects the two points X  $(\pi/a, \pi/a, 0)$  and P  $(\pi/a, \pi/a, \pi/a)$ . Along this W line, the twofold rotation is preserved and its

eigenvalues  $\pm 1$  remains constant, because the square of this rotation is  $+1$ . At the X point ( $\pi/a$ ,  $\pi/a$ , 0), the twofold rotation anticommutes with the inversion, which means that the twofold rotation eigenvalue changes sign under the inversion. Thus, at the X point, twofold degeneracy is formed by two states, one with  $C_{2z} = 1$  and the other with  $C_{2z} = -1$ . On the other hand, at the P point, all the eigenmodes are doubly degenerate with both sharing the same  $C_{2z}$  eigenvalue ( $=\pm 1$ ). This can be directly shown by the local symmetries at the P point,  $T' \equiv TG_y$  and  $IC_{4z}$ , with its details shown in the page 8 of the Supplementary Material of Ref. [11].

Let us recall that along the line  $W(\pi/a, \pi/a, k_z)$ , the  $C_{2z}$  eigenvalues are preserved. At the X point one state with  $C_{2z} = 1$  and another state with  $C_{2z} = -1$  are degenerate, but it cannot be connected to the double degeneracy at the P point, formed by the same value of the  $C_{2z}$  eigenvalues. Thus, in MSG **142.567**, minimal connectivity  $M$  must be larger than two, and a band gap cannot open between the bands 2 and 3.

## References

1. L. Lu, C. Fang, L. Fu, S. G. Johnson, J. D. Joannopoulos, and M. Soljačić, “Symmetry-protected topological photonic crystal in three dimensions,” *Nat. Phys.* 12, 337 (2016).
2. C. L. Kane and E. J. Mele, “ $Z_2$  topological order and the quantum spin Hall effect,” *Phys. Rev. Lett.* 95, 146802 (2005).
3. C. L. Kane and E. J. Mele, “Quantum spin Hall effect in graphene,” *Phys. Rev. Lett.* 95, 226801 (2005).
4. L. Fu, C. L. Kane, and E. J. Mele, “Topological insulators in three dimensions,” *Phys. Rev. Lett.* 98, 106803 (2007).
5. C. Fang and L. Fu, “New classes of three-dimensional topological crystalline insulators: Nonsymmorphic and magnetic,” *Phys. Rev. B* 91, 161105(R) (2015).
6. K. Shiozaki, M. Sato, and K. Gomi, “ $Z_2$  topology in nonsymmorphic crystalline insulators: Möbius twist in surface states,” *Phys. Rev. B* 91, 155120 (2015).
7. H. Kim, K. Shiozaki, and S. Murakami, “Glide-symmetric magnetic topological crystalline insulators with inversion symmetry,” *Phys. Rev. B* 100, 165202 (2019).
8. H. Kim and S. Murakami, “Glide-symmetric topological crystalline insulator phase in a nonprimitive lattice,” *Phys. Rev. B* 102, 195202 (2020).
9. T. Hahn, *International Tables for Crystallography, Volume A: Space Group Symmetry*, International Tables for Crystallography (Kluwer Academic Publishers, Dordrecht, Boston, London, 2002), 5th ed.
10. L. Lu, C. Fang, T. H. Hsieh, L. Fu, S. G. Johnson, J. D. Joannopoulos, and M. Soljačić, “Generalized three-dimensional Dirac points and  $Z_2$  gapless surface states in a topological photonic crystal,” *CLEO:2015 p. FTh3D.7*. (2015).
11. H. Cheng, Y. Sha, R. Liu, C. Fang, and L. Lu, “Discovering topological surface states of Dirac points,” *Phys. Rev. Lett.* 124, 104301 (2020).
12. M. I. Aroyo, J. M. Perez-Mato, C. Capillas, E. Kroumova, S. Ivantchev, G. Madariaga, A. Kirov, and H. Wondratschek, “Bilbao crystallographic server: I. databases and crystallographic computing programs,” *Zeitschrift für Kristallographie-Crystalline Materials* 221, 15–27 (2006).
13. L. Lu, L. Fu, J. D. Joannopoulos, and M. Soljačić, “Weyl points and line nodes in gyroid photonic crystals,” *Nature Photonics* 7, 294 (2013).
14. H. Watanabe and L. Lu, “Space group theory of photonic bands,” *Phys. Rev. Lett.* 121, 263903 (2018).
